# Supplementary material for: HG-PIPE: Vision Transformer Acceleration with Hybrid-Grained Pipeline
Source: arXiv:2407.17879 source file (2024-08-01)
Supplement: Supplementary file 1 [file 7-appendix.tex]

\section{Appendix}

\definecolor{loop1}{RGB}{255, 0, 0}
% Deep Sky Blue for loop2
\definecolor{loop2}{RGB}{0, 151, 205}
% Dark Orchid for loop3
\definecolor{loop3}{RGB}{153, 50, 204}
% Dark green for loop4
\definecolor{loop4}{RGB}{0, 150, 0}

\begin{algorithm}[htbp]
  \caption{Convolutional Algorithm}
  \label{alg:convolution}
  \begin{algorithmic}[1]
    \scriptsize
    \Procedure{Step3MACs}{$\mathbf{x\_stream}$, $\mathbf{w}$, $\mathbf{y\_stream}$}
    %   \State{}
      \State{\textsc{Do tile loops:}}
      \For{$\code{hit} \gets 0$ \textbf{to} $\code{HIT}$, $\code{wit} \gets 0$ \textbf{to} $\code{WIT}$}                            \Comment{\textcolor{loop1}{Tile1}}
        \For{$\code{cot} \gets 0$ \textbf{to} $\code{COT}$}                                                                         \Comment{\textcolor{loop2}{Tile2}}
          \For{$\code{cit} \gets 0$ \textbf{to} $\code{CIT}$}                                                                       \Comment{\textcolor{loop3}{Tile3}}
            \State{\#pragma HLS pipeline II=1}
            % \State{}
            \State{Read $\mathbf{x} \ll \mathbf{x\_stream}$}
            \State{Init $\mathbf{y} \gets \mathbf{0}_\mathbf{y}$ \textbf{if} $\code{cit} = 0$}
            % \State{}
            \State{\textsc{Do unroll loops:} \textbf{for}(}
            \State{\hspace{\algorithmicindent}$\code{hop} \gets 0$ \textbf{to} $\code{HIP}$} \Comment{ \textcolor{loop1}{Unroll1}       }
            \State{\hspace{\algorithmicindent}$\code{wop} \gets 0$ \textbf{to} $\code{WIP}$} \Comment{ \textcolor{loop1}{Unroll1}       }
            \State{\hspace{\algorithmicindent}$\code{cop} \gets 0$ \textbf{to} $\code{COP}$} \Comment{ \textcolor{loop2}{Unroll2}       }
            \State{\hspace{\algorithmicindent}$\code{cip} \gets 0$ \textbf{to} $\code{CIP}$} \Comment{ \textcolor{loop3}{Unroll3}       }
            \State{\hspace{\algorithmicindent}$\code{kh} \gets 0$ \textbf{to} $\code{KH}$}   \Comment{ \textcolor{loop4}{FullyUnroll4}  }
            \State{\hspace{\algorithmicindent}$\code{kw} \gets 0$ \textbf{to} $\code{KW}$}   \Comment{ \textcolor{loop4}{FullyUnroll4}  }
            \State{\textbf{) do}}
              \State{\hspace{\algorithmicindent}\#pragma HLS unroll}
            %   \State{}
              \State{\hspace{\algorithmicindent}$\code{hip} \gets \code{hop}\cdot\code{HS}+\code{kh}$}
              \State{\hspace{\algorithmicindent}$\code{wip} \gets \code{wop}\cdot\code{WS}+\code{kw}$}
              \State{\hspace{\algorithmicindent}$\code{ci} \gets \code{cit}\cdot\code{CIP}+\code{cip}$}
              \State{\hspace{\algorithmicindent}$\code{co} \gets \code{cot}\cdot\code{COP}+\code{cop}$}
            %   \State{}
              \State{\hspace{\algorithmicindent}$\mathbf{y}[\code{cop}][\code{hop}][\code{wop}]$ +=}
              \State{\hspace{\algorithmicindent}\hspace{\algorithmicindent}$\mathbf{x}[\code{cip}][\code{hip}][\code{wip}]\times$}
              \State{\hspace{\algorithmicindent}\hspace{\algorithmicindent}$\mathbf{w}[\code{co}][\code{ci}][\code{kh}][\code{kw}]$}
            % \State{}
            \State{\textbf{end for}} 
            \EndFor                                                                         \Comment{ End \textcolor{loop3}{Tile3}      }
            % \State{}
            \State{Write $\mathbf{y} \gg \mathbf{y\_stream}$}
            % \State{}
        \EndFor                                                                             \Comment{ End \textcolor{loop2}{Tile2}      }
      \EndFor                                                                               \Comment{ End \textcolor{loop1}{Tile1}      }
    \EndProcedure

  \end{algorithmic}
\end{algorithm}

The re-parameterization formation in LSQ:
In Eq.[conv],[residual],[requant], $\mathbf{B}_\text{int}$ is reconstructed BN $\mu$ parameter, $\mathbf{R}_\text{int}$ is residual scaling factor. The integer residual activation needs to be scaled because the main branch and residual branch have different scaling factors. $\mathbf{S}$ is the reconstructed scaling factor fused with the BN scaling factor.
\begin{equation}
    \mathbf{y}_\text{int} = \mathbf{x}_\text{int}\otimes\mathbf{w}_\text{int}+\mathbf{B}_\text{int},\quad \mathbf{B}_\text{int}= \left\lceil\cfrac{\beta\cdot \sqrt{\sigma^2+\epsilon}-\mu\gamma}{\gamma s_\mathbf{x} s_\mathbf{w}}\right\rfloor
\end{equation}
\begin{equation}
\mathbf{y}_\text{int}\, += \lceil\mathbf{R}\cdot\mathbf{x}\rfloor,\quad \mathbf{R} = \left(\cfrac{\gamma s_\mathbf{x} s_\mathbf{w}}{\sqrt{\sigma^2+\epsilon}}\right)_\text{res} \Bigg/ \left(\cfrac{\gamma s_\mathbf{x} s_\mathbf{w}}{\sqrt{\sigma^2+\epsilon}}\right)_\text{main}
\end{equation}
\begin{equation}
\mathbf{x}_\text{int}' = \text{clamp}(\lceil \mathbf{S} \cdot \mathbf{y}_\text{int} \rfloor, Q_\text{min}, Q_\text{max}), \quad \mathbf{S}= \cfrac{\gamma s_\mathbf{x} s_\mathbf{w}}{s_\mathbf{y}\sqrt{\sigma^2+\epsilon}}
\end{equation}

\begin{equation}
    \label{conv}
    \mathbf{y}_\text{int} = \mathbf{x}_\text{int}\otimes\mathbf{w}_\text{int}+\mathbf{B}_\text{int}
\end{equation}
\begin{equation}
    \label{residual}
\mathbf{y}_\text{int}\, += \lceil\mathbf{R}\cdot\mathbf{x}\rfloor
\end{equation}
\begin{equation}
    \label{requant}
\mathbf{y}_\text{int} = \text{clamp}(\lceil \mathbf{S} \cdot \mathbf{CONV}_\text{int} \rfloor, Q_\text{min}, Q_\text{max})
\end{equation}
